# Supplementary material for: Exploring Uncertainty in Conditional Multi-Modal Retrieval Systems
Source: arXiv:1901.07702 source file (2019-01-23)
Supplement: Supplementary file 1 [file supp_mat.tex]

%\section{Acknowledgments}
%This work is sponsored by Honda Research Institute USA

\newcommand{\beginsupplement}{%
	\setcounter{table}{0}
	\renewcommand{\thetable}{S\arabic{table}}%
	\setcounter{figure}{0}
	\renewcommand{\thefigure}{S\arabic{figure}}%
}

\beginsupplement

\section{Supplementary Material}

This supplementary material provides additional details about the experiments settings and results.

\section{Person Re-Identification}

Person re-identification provides a standard benchmark for quantitatively evaluating our triplet loss casting. In the main paper, our approach achieves comparable state-of-the-art results with dropout rate $p=0.15$. To demonstrate our approach generality, we employed both vanilla triplet loss with normalized embedding, and the adaptive weighted triplet loss (AWTL) with unnormalized embedding. Our triplet loss casting in section 3.1 assumes a unit circle embedding. Yet, it is straight-forward to extend it for unnormalized embedding with soft margin as follows
\begin{align}\label{eq:tri_func}
& f_{tri}(x_i,y_i,z_i)= d_i \in [0,\infty[\\
&={ \left[D(\left\lfloor x_i \right\rfloor ,\left\lfloor y_i \right\rfloor )-D(\left\lfloor x_i \right\rfloor,\left\lfloor z_i \right\rfloor) \right]  }_{ + } \label{eq:tri_func_full}
%&={ \left[emb(x_i)+emb(y_i)-emd(z_i) \right]  }_{ + } \label{eq:tri_func_full}
\end{align}
where ${ \left[ . \right]  }_{ + }= max(0,.)$. $\left\lfloor. \right\rfloor$ and $D(,)$ are an unconstrained embedding and the Euclidean distance functions respectively. $f_{tri}(x_i,y_i,z_i)$ outputs $d_i=0$ if $y_i,x_i \in c_i$ and $z_i \in c_j$; and $d_i \rightarrow \infty$ if $z_i,x_i \in c_i$ and $y_i \in c_j$  s.t. $i \ne j$. 

Tables~\ref{tbl:market_dense_p01},~\ref{tbl:duke_dense_p01} ~\ref{tbl:market_dense_p02}, and ~\ref{tbl:duke_dense_p02} illustrate our approach stability using different dropout rates $p=\{0.1, 0.2\}$ and two triple toss variants on both Market-1501 and DukeMTMC-ReID. Beyond persistent improvements, two key findings are worth-noting. First, the Monte-Carlo (MC) sampling utility increases as the dropout rate increases. Second, high dropout rate either leads to network divergence or requires more iterations to converge. Table~\ref{tbl:duke_dense_p02} emphasizes this phenomena on DukeMTMC-ReID dataset with dropout rate $p=0.2$. Thus, a mid-range dropout rate $p$ is required to avoid divergence and maintain a useful uncertainty estimation.

%For a fair comparison against standard benchmark~\cite{}, 25000 training iterations are employed. 

\begin{table}[h]
	\centering
	\begin{tabular}{|l|c|c|c|}
		\hline
		Method          & mAp &  Top 1 & $\triangle$mAp \\ \hline \hline
		Tri-Dense  &   69.58 &   84.12 & -	 \\ \hline 
		\textbf{Tri-Dense+50 MC}  &  \textbf{70.05} &  \textbf{84.32}	& 0.47 \\ \hline \hline
		Tri-Dense+AWTL &   71.38 &   85.07	& - \\ \hline 
		\textbf{Tri-Dense+AWTL+50 MC} &  \textbf{72.15} &  \textbf{86.70} &	0.77 \\ \hline
	\end{tabular}
	\caption{Market-1501 quantitative evaluation with dropout rate $p=0.1$. Our approach highlighted in bold.}
	\label{tbl:market_dense_p01}
\end{table}

\begin{table}[h]
	\centering
	\begin{tabular}{|l|c|c|c|}
		\hline
		Method          & mAp &  Top 1 & $\triangle$mAp \\ \hline \hline
		Tri-Dense  &   60.20 &   77.11 & -	 \\ \hline 
		\textbf{Tri-Dense+50 MC}  &  \textbf{61.24} &  \textbf{78.28}	& 1.04 \\ \hline \hline
		Tri-Dense+AWTL &   63.53 &   79.98	& - \\ \hline 
		\textbf{Tri-Dense+AWTL+50 MC} &  \textbf{64.75} &  \textbf{80.30} &	1.22 \\ \hline
	\end{tabular}
	\caption{DukeMTMC-ReID quantitative evaluation with $p=0.1$.}
	\label{tbl:duke_dense_p01}
\end{table}

\begin{table}[h]
	\centering
	\begin{tabular}{|l|c|c|c|}
		\hline
		Method          & mAp &  Top 1 & $\triangle$mAp \\ \hline \hline
		Tri-Dense  &   66.88 &   81.74 & -	 \\ \hline 
		\textbf{Tri-Dense+50 MC}  &  \textbf{67.88} &  \textbf{82.48}	& 1.00 \\ \hline \hline
		Tri-Dense+AWTL &   69.25 &   84.41	& - \\ \hline 
		\textbf{Tri-Dense+AWTL+50 MC} &  \textbf{70.58} &  \textbf{84.65} &	1.33 \\ \hline
	\end{tabular}
	\caption{Market-1501 quantitative evaluation with $p=0.2$}
	\label{tbl:market_dense_p02}
\end{table}

\begin{table}[h]
	\centering
	\begin{tabular}{|l|c|c|c|}
		\hline
		Method          & mAp &  Top 1 & $\triangle$mAp \\ \hline \hline
		Tri-Dense &   57.70 &   74.82 & -	 \\ \hline 
		\textbf{Tri-Dense+50 MC}  &  \textbf{59.26} &  \textbf{76.44}	& 1.56 \\ \hline \hline
		Tri-Dense+AWTL &   27.59 &   42.95	& - \\ \hline 
		\textbf{Tri-Dense+AWTL+50 MC} &  \textbf{32.04} &  \textbf{47.89} &	4.45 \\ \hline
	\end{tabular}
	\caption{DukeMTMC-ReID quantitative evaluation with $p=0.2$.}
	\label{tbl:duke_dense_p02}
\end{table}

\section{Autonomous Car Driving}
\subsection{Architecture Details}
Figure~\ref{fig:arch} shows the architecture employed in the autonomous navigation experiment.
Table~\ref{tbl:arch_params} present the inputs and trainable layers dimensions. Video frames are represented using pre-extracted features from the Conv2d\_7b\_1x1 layer of InceptionResnet-V2~\cite{szegedy2017inception} pretrained on ImageNet -- ResNet features.

\begin{figure*}[ht!]
	\begin{center}
		\includegraphics[width=0.8\linewidth]{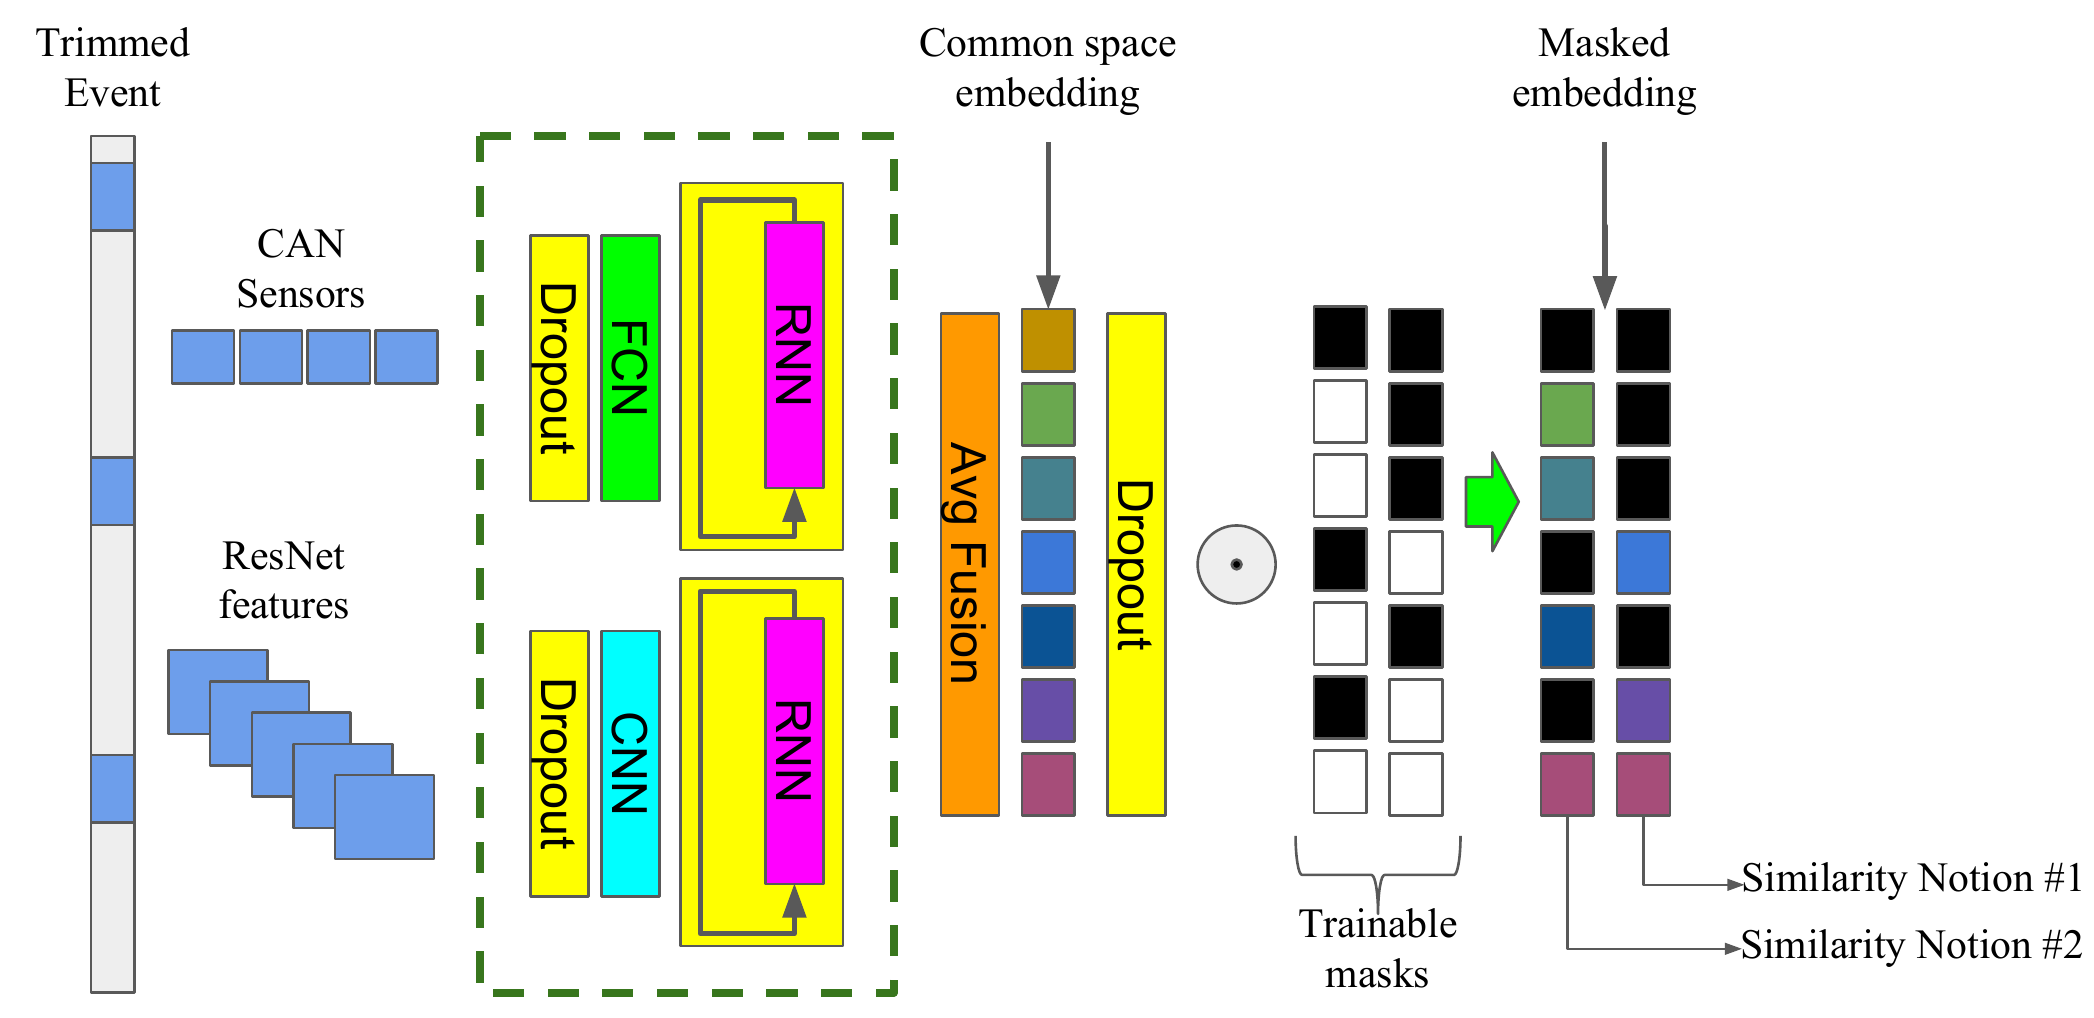}
	\end{center}
	
	\caption{Our proposed multi-modal conditional retrieval end-to-end network. Given a trimmed event, multiple samples are drawn. ResNet features, pre-extracted from video frames, and CAN sensors are independently embedded using separate encoders; then fused into a common space by averaging. Trainable masks enable conditional retrieval for the multiple similarity notions.}
	\label{fig:arch}
\end{figure*}

\begin{table*}[h]
	\centering
	\begin{tabular}{|l|l|l|l|}
		\hline
		Layer/Input         & Input Dimension & Layer Dimension & Output \\ \hline
		CAN sensor       & $8$     & N/A & N/A \\ \hline
		FCN & $8$ & $8\times128$ & $128$ \\ \hline
		RNN (CAN) & $N\times128$ & $128$  & $128$\\ \hline \hline

		ResNet features & $8\times8\times1536$     & N/A & N/A \\ \hline
		CNN Kernel & $8\times8\times1536$ & $1\times1\times1536\times20$ & $8\times8\times20$ \\ \hline
		RNN (ResNet) & $N\times1280$ & $128$ & $128$ \\ \hline \hline
		Mean Fusion & $2\times128$ & N/A & $128$ \\ \hline 
		Trainable masks & $128$ & $M\times128$ & $M\times128$ \\ \hline
	\end{tabular}
	\caption{$N$ indicates the number of samples drawn from an event for temporal fusion. $M$ indicates the number of similarity notions. Bias weights are omitted. In our experiments, $N=3$ and $M=2$.}
	\label{tbl:arch_params}
\end{table*}

\subsection{Dataset details}
The Honda driving dataset (HDD) records 104 hours of real human driving in the San Francisco Bay Area using an instrumented vehicle.  The recording consists of 137 sessions $S$, and each session $S_i$ represents a navigation task performed by a driver. The training, validation and testing splits contain 93, 5, and 36 sessions respectively. Three sessions are omitted for missing annotations or CAN sensors signals. %The average duration of each session is 45 minutes. Figure~\ref{fig:hdd_stats} presents session durations  statistics.

\begin{comment}

\begin{figure}[h!]
	\begin{tikzpicture} 
	\begin{axis}[ ybar,width=0.5\textwidth, height=4.5cm, enlargelimits=0.15, xtick=data, nodes near coords align={vertical}, x tick label style={rotate=45,anchor=east},] 
	
	\addplot coordinates {
		(12,33) 
		(29,39) 
		(45,17) 
		(62,20) 
		(78,14) 
		(95,4) 
		(111,5) 
		(128,3) 
		(144,0) 
		(166,2)
	};  \end{axis}
	\end{tikzpicture}
	\caption{HDD sessions duration histogram. X-axis indicates the bin center in mins; y-axis in the number of sessions within the bin}
	\label{fig:hdd_stats}
\end{figure}

\end{comment}
% More HDD dataset details

% Why dropout 0.1

% AWTL Triplet lost casting extension

% How do you know more samples boost performance.

%HDD has four annotation layers to explain the drivers' actions: Goal-oriented, stimulus-driven, cause and attention. The \textbf{Goal-oriented} layer, utilized in our experiments , defines drivers' actions to reach their destinations, \eg left-turn and intersection passing.~\cite{ramanishka2018toward} provides further details for the other three annotation layers.

Schroff \etal~\cite{schroff2015facenet} promote a large batch size for an efficient triplet loss convergence. In our experiments, $N_{Tri}=400$ is utilized during training. To avoid GPU memory limitations, video frames are represented using pre-extracted ResNet features. This reduces the neural network size and allows a large number of triplets.
%We adopt a compact, but efficient, network architecture and 

HDD suffers class imbalance. Random sampling is inadequate for creating the triplet loss training batches. We present our batch construction and training procedure in algorithm~\ref{alg:sampling}. First, three sessions $S_\phi$ are randomly sampled from $S$. Using multiple feed-forwards, action embeddings $E_A$ are computed, where $A$ are the drivers' actions in $S_\phi$. Then, the pairwise distance matrix $D_A$ between actions $A$ is computed using $E_A$.  The training triplets utilize all positive pairs and their corresponding semi-hard negative samples. This process repeats till all sessions are sampled during each epoch.

%Finally, all positive action pairs are constructed and semi-hard negative samples are identified using the pairwise distance matrix.

% To avoid GPU memory limitation, the number of generated triplet is constrained to $N_{Tri}$. 

In the main paper, we intuitively argue about goal-oriented verses stimulus-driven retrieval uncertainty. We attribute the  stimulus-driven high uncertainty to CAN sensors visual limitations. Table~\ref{tbl:var_map} provides quantitative evaluation for retrieval uncertainty. The mean variance, across all embeddings, normalized by the number of classes is reported. The mAp improvements ($\triangle$ mAp) are reported from tables 3 and 4 in the main paper. These results align with our claims, i.e. a positive correlation between the system uncertainty and MC sampling utility.

\begin{comment}
Quantitative uncertainty estimation can be misleading. In a binary imbalance classification problem, \eg the majority class represents 98\% of the data, an inferior system will always predict the majority class with zero variance. The number of classes and their distribution are key factors affecting system uncertainty. This explains why we focused on the intuitive arguments in the main paper.
\end{comment}

\begin{table}[ht]
	\begin{center}
		\begin{tabular}{|l|c|c|}
			\hline
			 & Var & $\triangle$ mAp \\ \hline
			Goal & $2.30 *10^{-3}$ &  0.23 \\ \hline
			Stimulus & $3.54 *10^{-3}$ &  6.26 \\ \hline
		\end{tabular}
	\end{center}
	\caption{Model Uncertainty and the corresponding mAp improvement for goal-oriented verses stimulus-driven retrieval. As the task uncertainty increases, MC sampling achieves larger improvement.}
	\label{tbl:var_map}
\end{table}
%Our approach perform best in high uncertainty environment -- event retrieval using stimulus.

 %feed-forwards, $E_A$ embedding .
%Stack of difference (SOD) encodes the driver actions.  This enables computing pairwise distance matrix between actions. 

Figure~\ref{fig:sub_qual_eval} presents a further qualitative evaluation on HDD. It shows three queries highlighted in blue, followed by their top two retrieval results. Correct and incorrect results are highlighted in green and red respectively. The first two queries are slow, and careful, \textit{left-turn} and \textit{right-turn} maneuvers affected by pedestrians or opposite traffic. The last query is a \textit{U-turn} maneuver where the second retrieval result is an incorrect \textit{left-turn}. \textit{U-Turn} is a minority class often confused with \textit{left-turn}. Better visualizations using GIFs are attached. %Upon submission acceptance, visualizations using GIFs will be released online.

\begin{algorithm}[h]
	%	\scriptsize
	\caption{HDD training and triplets construction procedure. In our experiments, $b=512$ is the mini-batch size, $N_{Tri}=400$ is the maximum number of triplets, and $N_{epoch} =500$ is the number of epochs.}
	\begin{algorithmic}
		\REQUIRE $S$ is the driving training sessions
		\REQUIRE $T_{tri}$ stores the training triplets
		\REQUIRE $E_A$ stores action embeddings
		\FOR{e in $N_{epoch}$} 
		\STATE load training sessions $S$
		\WHILE {$S$ \textbf{is not} empty}
			\STATE Draw three driving sessions $S_\phi$ from $S$
			\STATE Load $S_\phi$ actions $A$ 
			\STATE // Multiple feed-forwards to compute $E_A$
			\FOR {$i=0$ \TO $len(A)//b$}
				\STATE $A_b = A[i*b:(i+1)*b]$
				\STATE Compute $E_A[i*b:(i+1)*b]$ for $A_b$
			\ENDFOR
			\STATE Compute pairwise distance matrix $D_A$ using $E_A$
			\STATE $T_{tri} = \Phi$
			\STATE Construct all positive pairs $pos\_prs$
			\FORALL{$(a,p)$ in $pos\_prs$} 
			\STATE Find nearest semi-hard negative $n$ using $D_A$ 
			\STATE append $(a,p,n)$ to $T_{tri}$
			\ENDFOR
			\IF {$len(T_{tri}) > N_{Tri} $}
			\STATE $T_{tri} = shuffle(T_{tri})[0:N_{Tri}]$
			\ENDIF
			\STATE // $T_{tri}$ contains $N_{Tri}$ triplets $(a,p,n)$
			\STATE Feed-forward  $T_{tri}$
			\STATE Compute triplet loss then back-propagate.
			\ENDWHILE
		\ENDFOR

	\end{algorithmic}
	\label{alg:sampling}
\end{algorithm}

%\subsection{Evaluations}

\begin{figure*}[t!]
	\begin{subfigure}{1.0\textwidth}
		\centering
		\setlength{\fboxsep}{0pt}%
		\setlength{\fboxrule}{2pt}%
		
		\fcolorbox{blue}{white}{\includegraphics[width=.19\linewidth]{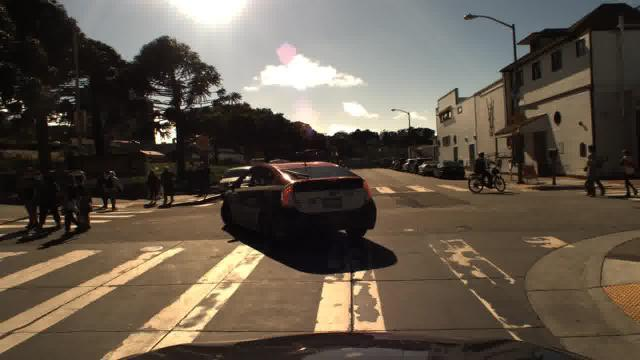}
			\includegraphics[width=.19\linewidth]{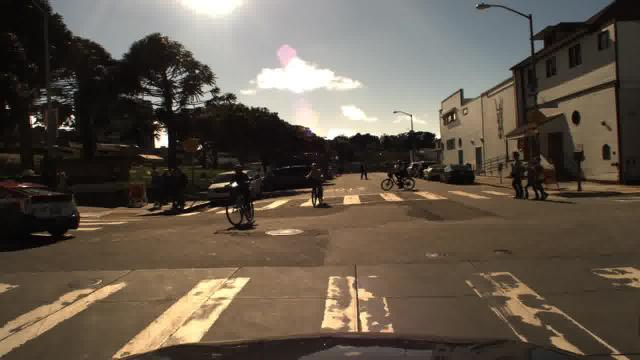}
			\includegraphics[width=.19\linewidth]{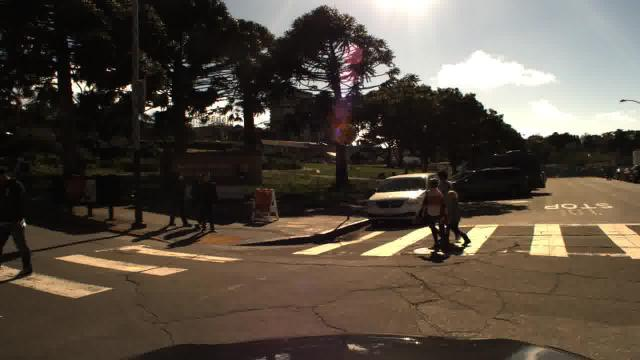}
			\includegraphics[width=.19\linewidth]{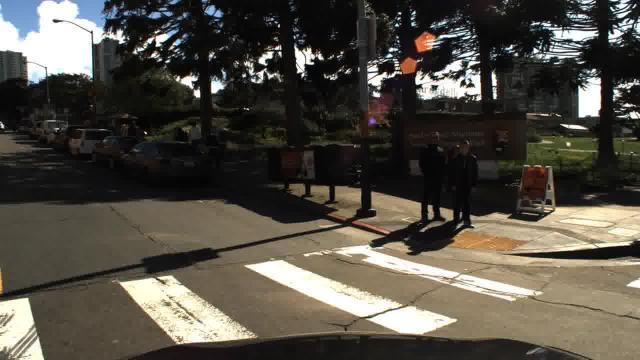}
			\includegraphics[width=.19\linewidth]{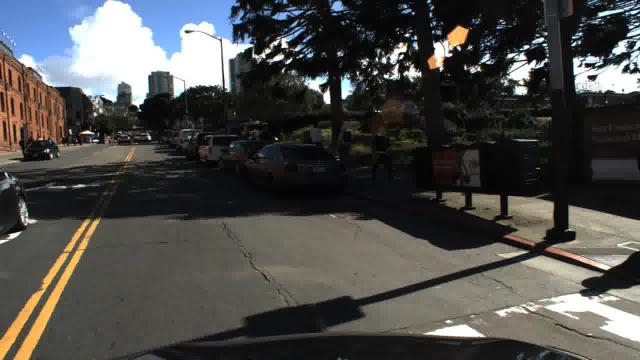}}
	\end{subfigure}
	\begin{subfigure}{1.0\textwidth}
		\centering
		\setlength{\fboxsep}{0pt}%
		\setlength{\fboxrule}{2pt}%
		\fcolorbox{green}{white}{\includegraphics[width=.19\linewidth]{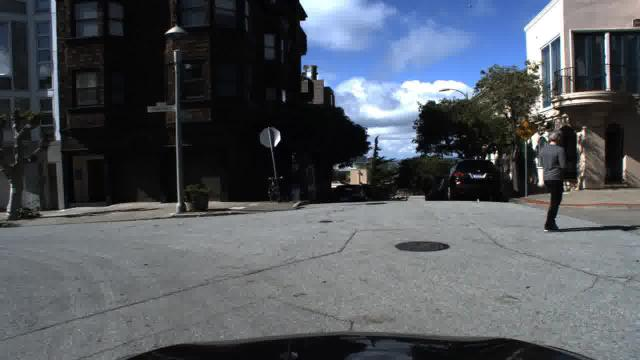}
			\includegraphics[width=.19\linewidth]{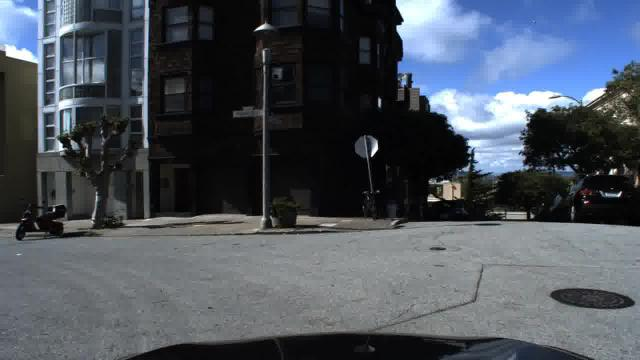}
			\includegraphics[width=.19\linewidth]{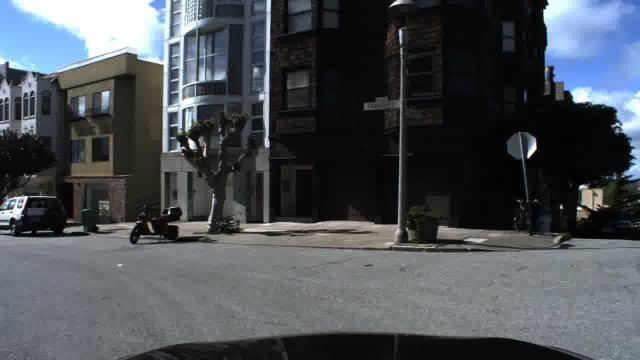}
			\includegraphics[width=.19\linewidth]{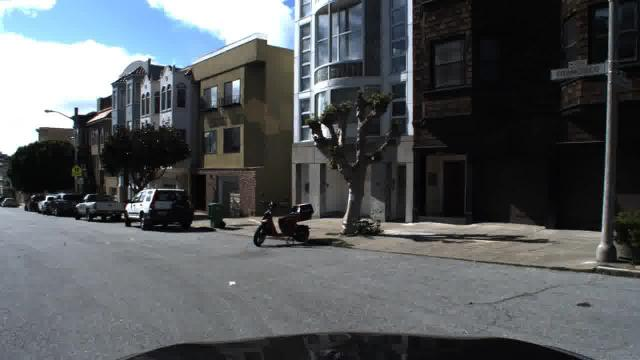}
			\includegraphics[width=.19\linewidth]{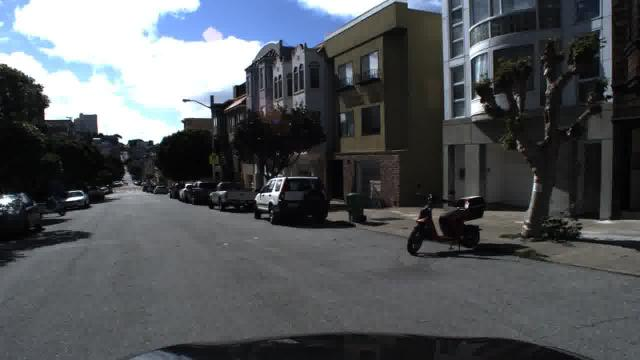}}
	\end{subfigure}
	\begin{subfigure}{1.0\textwidth}
		\centering
		\setlength{\fboxsep}{0pt}%
		\setlength{\fboxrule}{2pt}%
		\fcolorbox{green}{white}{\includegraphics[width=.19\linewidth]{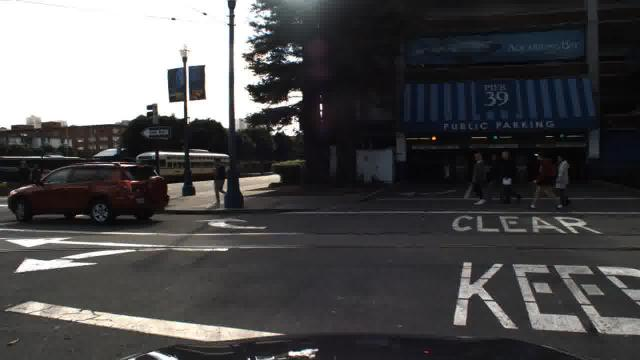}
			\includegraphics[width=.19\linewidth]{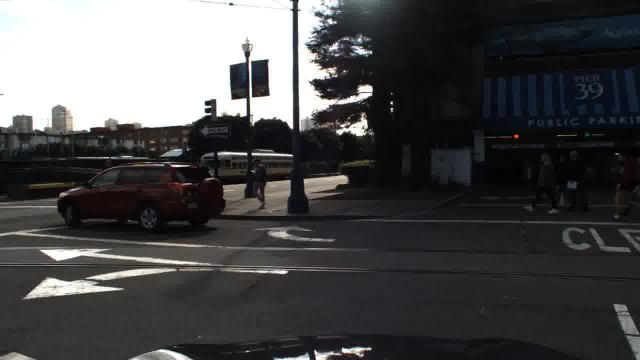}
			\includegraphics[width=.19\linewidth]{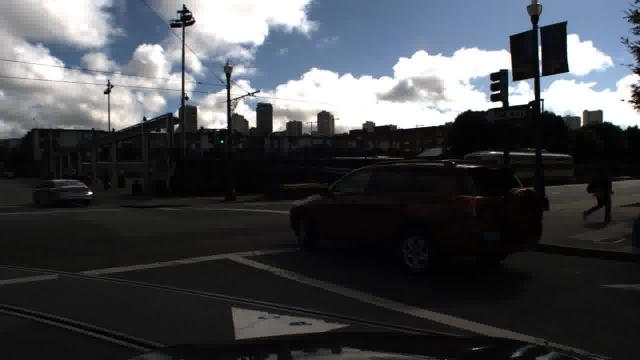}
			\includegraphics[width=.19\linewidth]{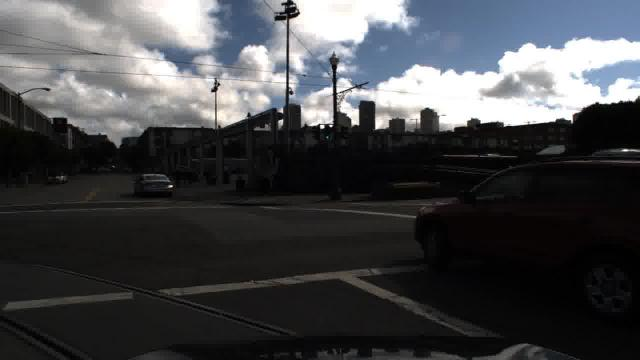}
			\includegraphics[width=.19\linewidth]{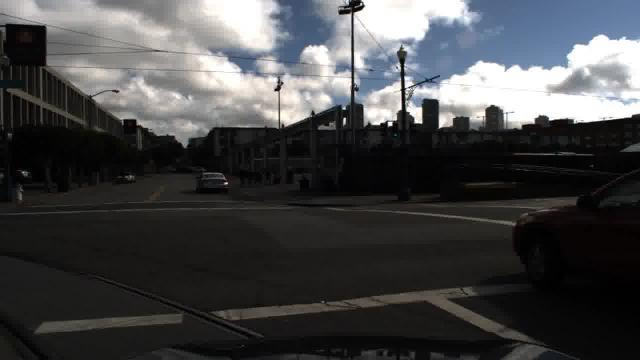}}
	\end{subfigure}

\begin{subfigure}{1.0\textwidth}
			\centering
	\setlength{\fboxsep}{0pt}%
	\setlength{\fboxrule}{2pt}%
		\fcolorbox{blue}{white}{\includegraphics[width=.19\linewidth]{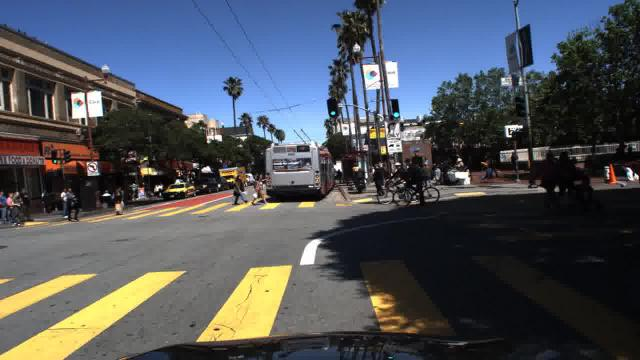}
	\includegraphics[width=.19\linewidth]{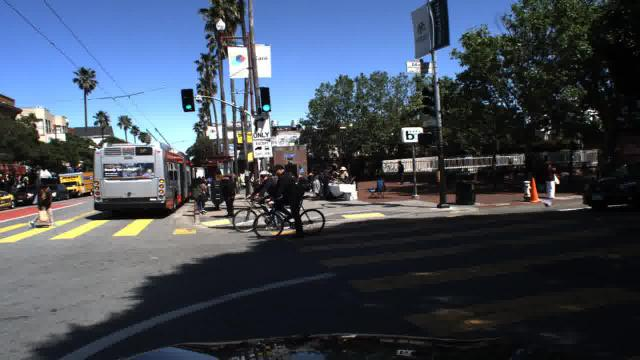}
	\includegraphics[width=.19\linewidth]{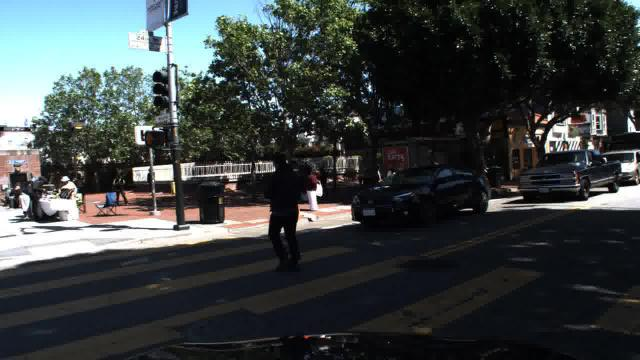}
	\includegraphics[width=.19\linewidth]{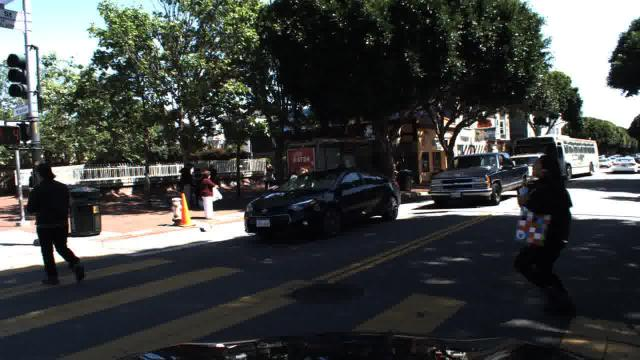}
	\includegraphics[width=.19\linewidth]{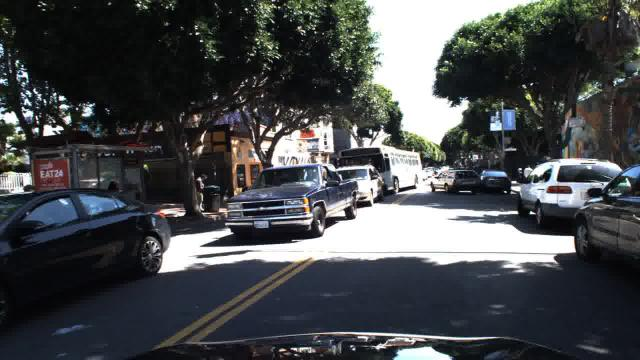}}
\end{subfigure}

\begin{subfigure}{1.0\textwidth}
	\centering
	\setlength{\fboxsep}{0pt}%
	\setlength{\fboxrule}{2pt}%
	\fcolorbox{green}{white}{\includegraphics[width=.19\linewidth]{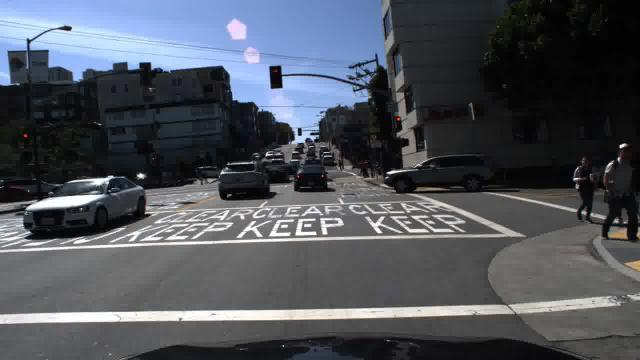}
		\includegraphics[width=.19\linewidth]{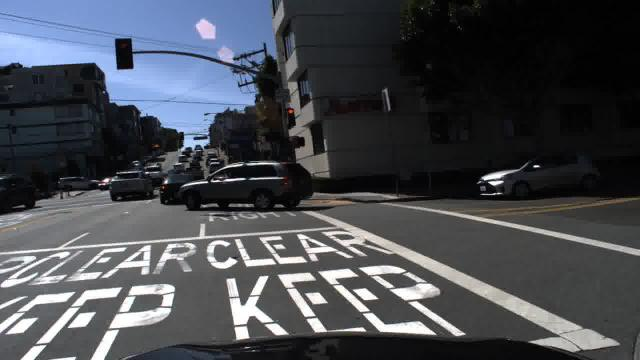}
		\includegraphics[width=.19\linewidth]{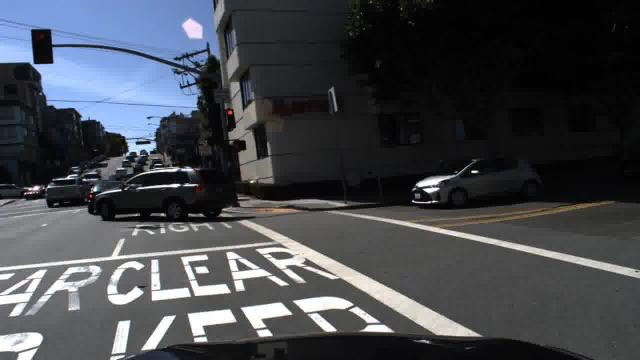}
		\includegraphics[width=.19\linewidth]{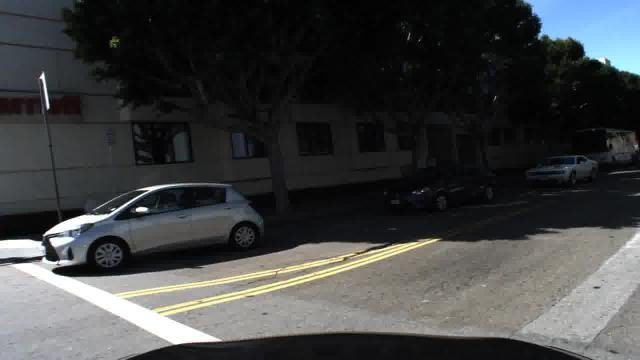}
		\includegraphics[width=.19\linewidth]{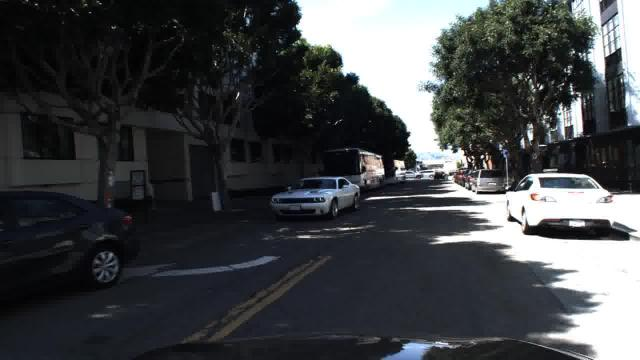}}
\end{subfigure}

\begin{subfigure}{1.0\textwidth}
	\centering
	\setlength{\fboxsep}{0pt}%
	\setlength{\fboxrule}{2pt}%
	\fcolorbox{green}{white}{\includegraphics[width=.19\linewidth]{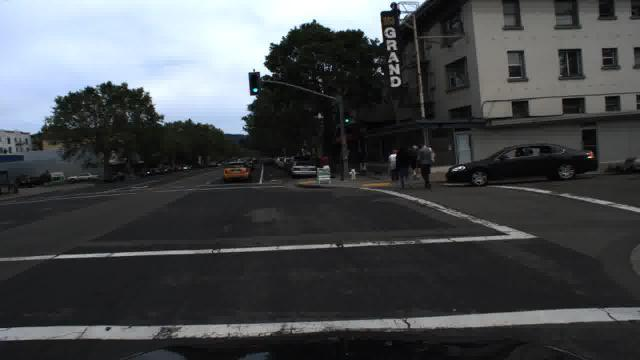}
		\includegraphics[width=.19\linewidth]{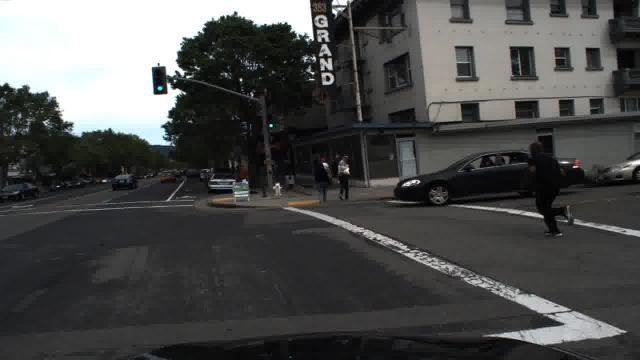}
		\includegraphics[width=.19\linewidth]{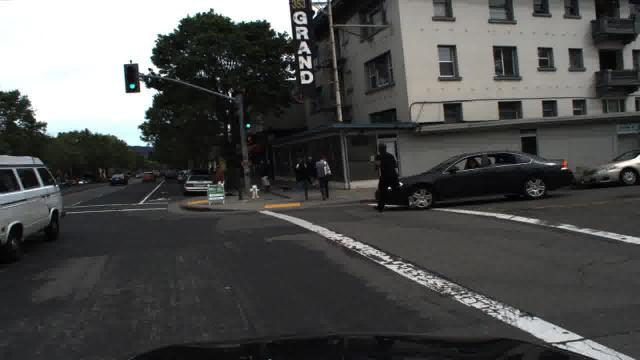}
		\includegraphics[width=.19\linewidth]{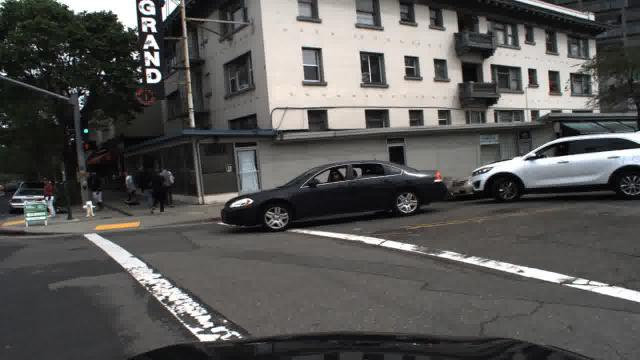}
		\includegraphics[width=.19\linewidth]{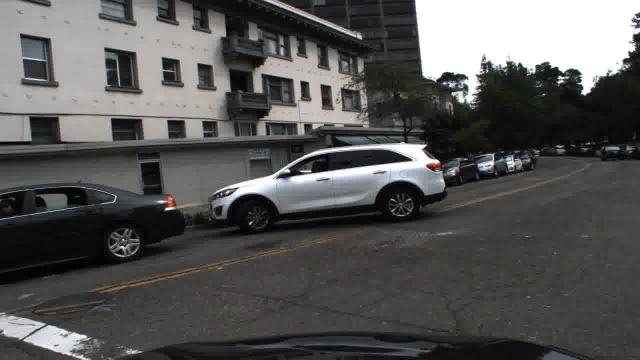}}
\end{subfigure}

\begin{subfigure}{1.0\textwidth}
	\centering
	\setlength{\fboxsep}{0pt}%
	\setlength{\fboxrule}{2pt}%
	\fcolorbox{blue}{white}{\includegraphics[width=.19\linewidth]{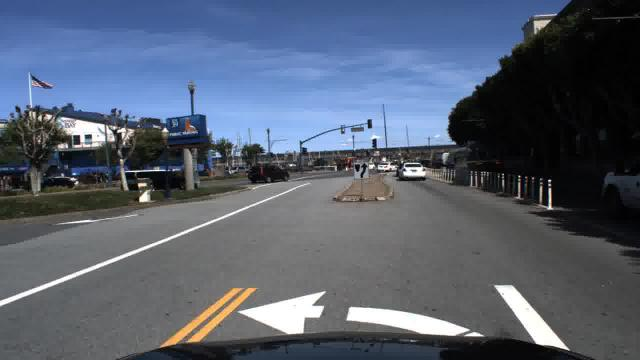}
		\includegraphics[width=.19\linewidth]{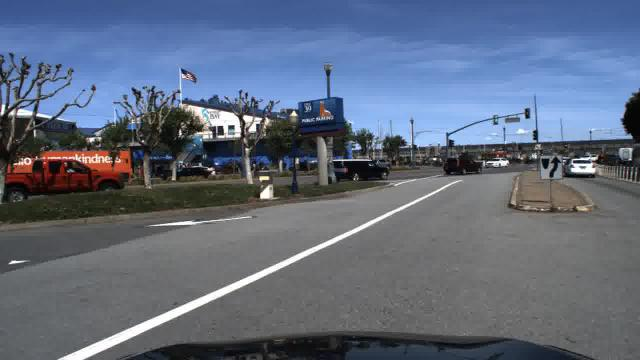}
		\includegraphics[width=.19\linewidth]{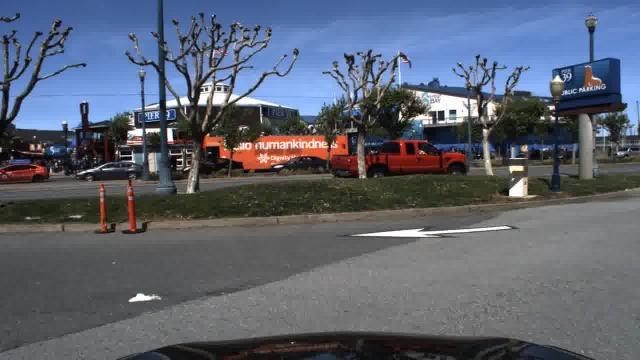}
		\includegraphics[width=.19\linewidth]{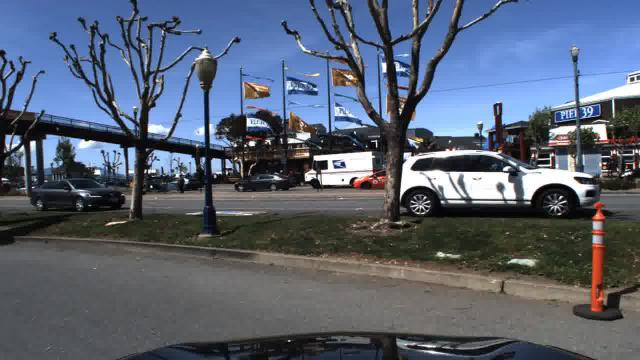}
		\includegraphics[width=.19\linewidth]{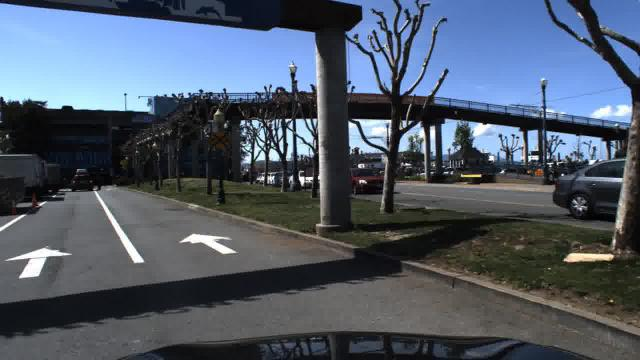}}
\end{subfigure}

\begin{subfigure}{1.0\textwidth}
	\centering
	\setlength{\fboxsep}{0pt}%
	\setlength{\fboxrule}{2pt}%
	\fcolorbox{green}{white}{\includegraphics[width=.19\linewidth]{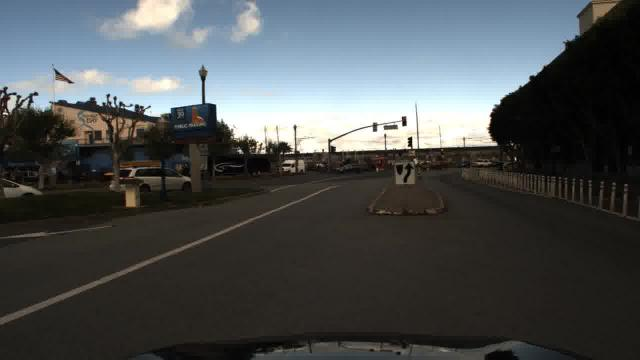}
		\includegraphics[width=.19\linewidth]{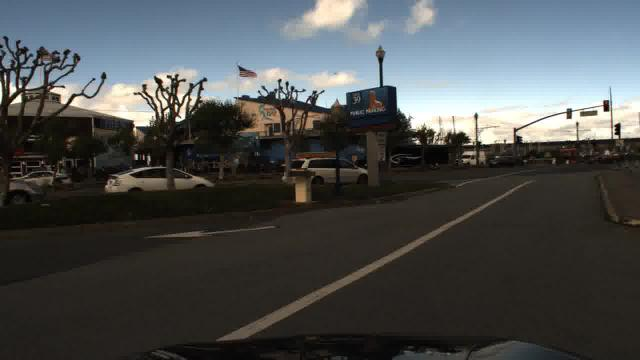}
		\includegraphics[width=.19\linewidth]{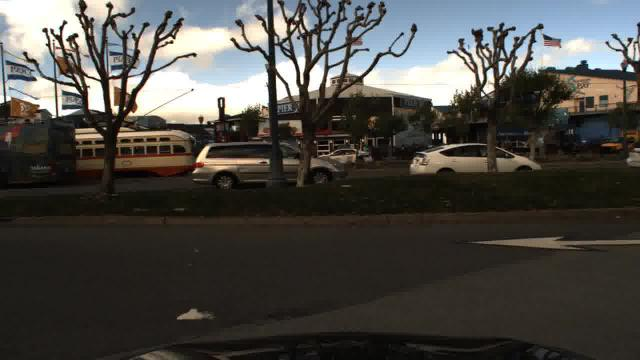}
		\includegraphics[width=.19\linewidth]{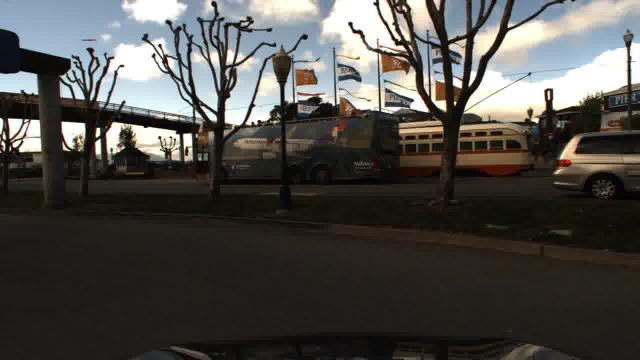}
		\includegraphics[width=.19\linewidth]{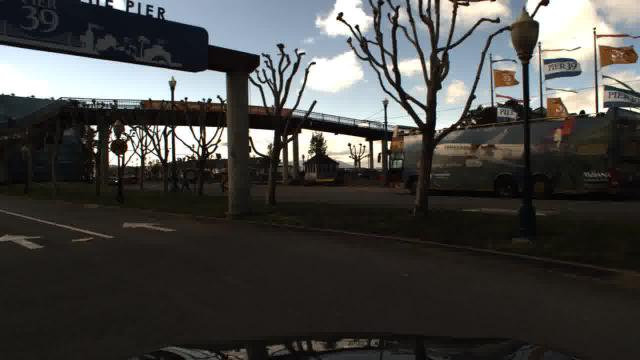}}
\end{subfigure}

\begin{subfigure}{1.0\textwidth}
	\centering
	\setlength{\fboxsep}{0pt}%
	\setlength{\fboxrule}{2pt}%
	\fcolorbox{red}{white}{\includegraphics[width=.19\linewidth]{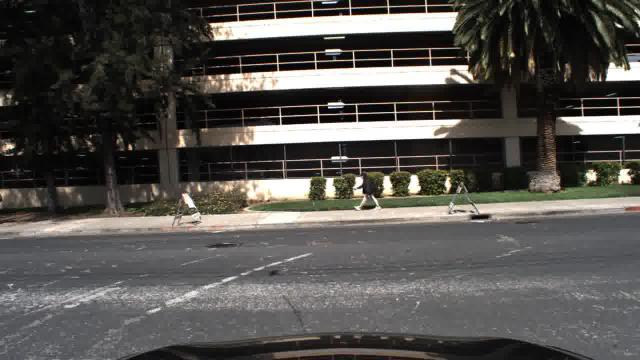}
		\includegraphics[width=.19\linewidth]{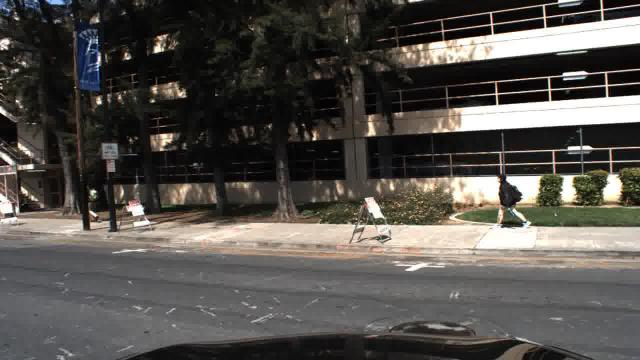}
		\includegraphics[width=.19\linewidth]{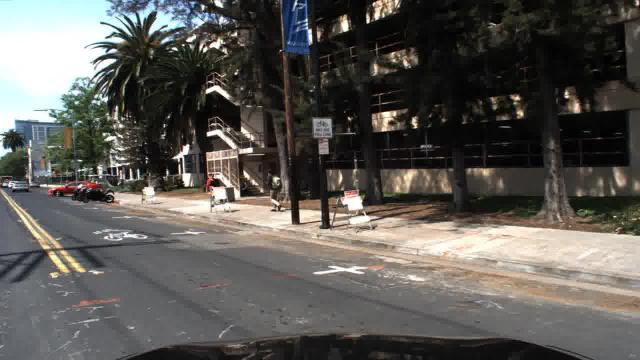}
		\includegraphics[width=.19\linewidth]{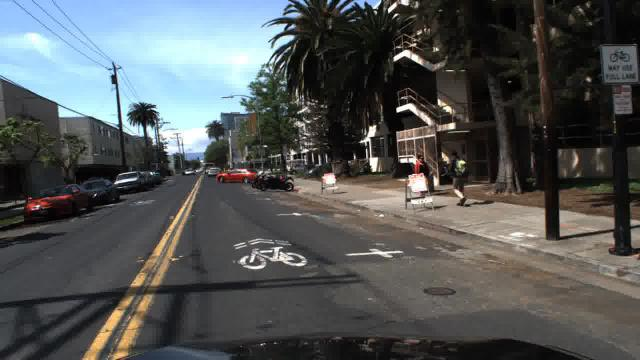}
		\includegraphics[width=.19\linewidth]{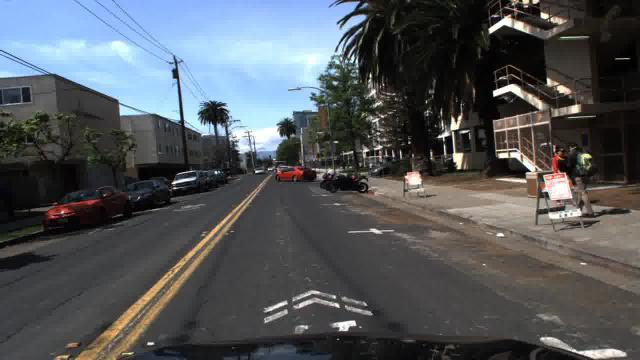}}
\end{subfigure}

\begin{comment}
	\begin{subfigure}{1.0\textwidth}
	\centering
	\setlength{\fboxsep}{0pt}%
	\setlength{\fboxrule}{2pt}%
	\fcolorbox{blue}{white}{\includegraphics[width=.19\linewidth]{sub_figures/left_turn_21/q21_1404}
	\includegraphics[width=.19\linewidth]{sub_figures/left_turn_21/q21_1407}
	\includegraphics[width=.19\linewidth]{sub_figures/left_turn_21/q21_1409}
	\includegraphics[width=.19\linewidth]{sub_figures/left_turn_21/q21_1411}
	\includegraphics[width=.19\linewidth]{sub_figures/left_turn_21/q21_1413}}
	\end{subfigure}
\end{comment}

\caption{Qualitative evaluation using three query events highlighted in blue. Every query is followed by the top two retrieval results. Correct and incorrect results are highlighted in green and red respectively. These queries emphasize various action classes: left, right and U turns. These images are best viewed in color/screen.}
\label{fig:sub_qual_eval}

\end{figure*}
