# Supplementary material for: Exploring Uncertainty in Conditional Multi-Modal Retrieval Systems
Source: arXiv:1901.07702 source file (2019-01-23)
Supplement: Supplementary file 2 [file appendix.tex]

%\begin{appendices}
\appendix
\section{Architecture details}
\label{appendix:arch}

\section{Dataset Details}
\label{appendix:dataset}
\begin{figure}[h]
	\begin{tikzpicture} 
	\begin{axis}[ ybar,width=0.5\textwidth, height=4.5cm, enlargelimits=0.15, xtick=data, nodes near coords align={vertical}, x tick label style={rotate=45,anchor=east},] 
	
	\addplot coordinates {
		(12,33) 
		(29,39) 
		(45,17) 
		(62,20) 
		(78,14) 
		(95,4) 
		(111,5) 
		(128,3) 
		(144,0) 
		(166,2)
	};  \end{axis}
	\end{tikzpicture}
	\caption{HDD sessions duration histogram. X-axis indicates the bin center in mins; y-axis in the number of sessions within the bin}
	\label{fig:sess_hist}
\end{figure}

%\end{appendices}
